# Supplementary material for: Iterative Deployment Exposure for Unsupervised Out-of-Distribution Detection
Source: arXiv:2406.02327 source file (2025-05-19)
Supplement: Supplementary file 1 [file 07appendix.tex]

\section{Supplementary Material}

\begin{table*}[t]
\centering
\setlength{\tabcolsep}{3pt}
\begin{tabular}{lccccccccccc}
\toprule
& \multirow{2}{*}{Plane}  & \multirow{2}{*}{Car} & \multirow{2}{*}{Bird} & \multirow{2}{*}{ Cat} & \multirow{2}{*}{Deer}  & \multirow{2}{*}{Dog}   & \multirow{2}{*}{Frog} & \multirow{2}{*}{Horse}  & \multirow{2}{*}{Ship}  & \multirow{2}{*}{Truck}   & \multirow{2}{*}{Mean} \\
\\
\midrule
SAL & 61.8	&	83.3	&	59.1	&	62.1	&	64.7	&	65.3	&	74.2	&	68.9	&	76.1	&	86.0	&	70.2\\
HSC & 82.6	&	81.0	&	64.7	&	72	&	71.5	&	70.7	&	82.0	&	78.7	&	87.2	&	86.0	&	77.6\\
ETLT & 87.4	&	94.2	&	81.2	&	81.5	&	91.7	&	84.6	&	90.8	&	89.3	&	93.9	&	94.8	&	89.0 \\
MahaAD & 88.0	&	93.2	&	80.1	&	79.7	&	91.1	&	84.9	&	90.5	&	89.4	&	93.1	&	95.0	&	88.5\\
BCE & 85.1	&	89.5	&	79.9	&	78.4	&	83.4	&	80.3	&	90.2	&	82.1	&	90.2	&	89.7	&	84.9\\
AdaODD & 92.0	&	\textbf{96.6}	&	\textbf{87.7}	&	86.7	&	\textbf{94.0}	&	\textbf{91.5}	&	\underline{94.5}	&	\textbf{95.4}	&	\underline{95.5}	&	\textbf{97.5}	&	\textbf{93.1}\\
MDiff & \underline{93.0}	&	94.3	&	\underline{84.6}	&	81.3	&	92.2	&	88.4	&	93.8	&	91.1	&	95.1	&	95.8	&	91.0\\
\rowcolor{mygray} \textbf{ours} & \textbf{93.1}	&	\underline{95.5}	&	\textbf{87.7}	&	\underline{84.9}	&	\underline{93.2}	&  \underline{90.7}	&	\textbf{95.4}	&	\underline{95.1}	&	\textbf{96.0}	&	\underline{96.6}	&	\underline{92.8}\\
\bottomrule
\end{tabular}
\caption{\textbf{Comparative evaluation on \oc.} We report the mean of the AUA ($\uparrow$) over five trials. \textbf{Bold} and \underline{underlined} indicate best and second best, respectively. Our method is among the two best methods for all cases.}
\label{tab:oneclassaua}
% }
\end{table*}

\subsection{Baseline Details}

We briefly describe all baselines and their hyperparameter ranges considered in the grid search. The ranges are based on the values found in each method's original publication. To adapt them to the continual U-OOD setting, we apply the baselines sequentially, pseudo-labeling new samples with the model from the previous timestep. Further method-specific adaptations, if any, are detailed below. All methods use a ResNet18 pre-trained on ImageNet with images resized to $224\times{}224$. 
\begin{description}
    \item[HSC~\cite{liznerski2022exposing}] aims to obtain compact representations for ID samples while pushing features of anomalous samples further away. We search over the learning rate $lr\in[1e^{-4},1e^{-5},1e^{-6}]$, and pseudo-labeling threshold $\tau\in[80,90,95,98]$. The threshold is a percentage such that $\tau\%$ of the training data is considered in-distribution. The best-performing configuration was $lr=1e^{-6}, \tau=80$.
    \item[ETLT~\cite{fan2022simple}] computes OOD scores for all available samples with a standard OOD detector, then fits linear regression to features extracted from a trained classifier to predict these scores. PCA is used to reduce the dimensionality of the feature vectors. We use MahaAD to compute the initial OOD scores to predict and swap the classifier for a pre-trained network. We search over the dimensionality $d\in[64,128,256,512]$. The best-performing configuration was $d=256$.
    \item[MahaAD~\cite{rippel2021modeling}] scores samples by summing the Mahalanobis distances to the training mean per layer. Used as a U-OOD baseline and comes without hyperparameters. 
    \item[BCE~\cite{liznerski2022exposing}] trains a binary classifier at every step and pseudo-labels samples with the resulting model. The exception is the first step, where we rely on MahaAD as the base detector. We search over the learning rate $lr\in[1e^{-4},1e^{-5}]$, OOD oversampling factor $oof\in[10,50]$, and pseudo-labeling threshold $\tau\in[80,90,95]$. The best-performing configuration was $lr=1e^{-5}, oof=10, \tau=90$.
    \item[SAL~\cite{du2024does}] finds candidate OOD samples based on their gradients with respect to the predicted label using a trained classifier, then trains a binary ID/OOD classifier together with the standard empirical risk minimization loss. We swap out the classifier for the pre-trained network and only train the binary classifier, as we do not have access to class labels. We search over the number of singular vectors $c\in[1,2,5,10,128,256,512]$ and use the same training settings as BCE. The best-performing configuration was $c=512, lr=1e^{-5}, oof=10, \tau=90$.
    \item[AdaODD~\cite{zhang2023model}] keeps a memory bank of normalized features extracted from a classifier. It scores samples with a kNN score. Confidently pseudo-labeled test samples are added to the memory bank. We swap the classifier for the pre-trained network. We search over the number of neighbors $k\in[2,10,50]$, selection margin $\gamma\in[1,1.5,2]$, and OOD scaling factor $\kappa\in[2,5,10,50]$. The best-performing configuration was $k=2, \gamma=2, \kappa=5$.
    \item[MDiff~\cite{sehwag2021ssd}] models both the in- and out-distribution as a Gaussian and scores samples by the distance to the in-distribution minus the distance to the out-distribution. We use a multi-scale version with the pre-trained network using the same layers as MahaAD and our method. We search over the threshold $\tau$ used to pseudo-label incoming test samples. We search over $\tau\in[80,85,90,95,98]$. The best-performing configuration was $\tau=85$.
    \item[Ours.] We search over $\beta$, influencing the mixing of $s^-$ and $s^+$, in $\beta\in[1/100,1/300,1/500]$, and over $\gamma$, influencing the uncertainty scaling, in $\gamma\in[1,3,5]$, and the pseudo-labeling threshold $\tau\in[80,90,95]$. The best-performing configuration was $\beta=100, \gamma=5, \tau=95$. Other hyperparameters were set as follows: the shrinkage is found using the standard hyperparameter-free Ledoit-Wolf estimator. The bootstrap estimate converges quickly with the number of samples, which was set to a sufficiently large value of~100. $k$~is set to 2, as is standard in U-OOD (e.g., \cite{reiss2023mean}).
\end{description}

\subsection{\oc~AUA Results}

We provide the AUA results on \oc~in \cref{tab:oneclassaua}, which gives similar conclusions as the AUF in \cref{tab:oneclass}, except for AdaODD scoring comparatively better and BCE scoring comparatively worse. Our method performs well and is the only method to score in the top two for all ten experiments.

\subsection{Larger Architectures}

We compare our method to the second-best method MDiff on \oc~with newer and larger architectures, a ConvNext-s and a ViT-B. From Tab.~\ref{tab:oneclass}, we also outperform MDiff with these larger architectures.

\begin{table*}[h]
\centering
\setlength{\tabcolsep}{3pt}
\begin{tabular}{lccccccccccc}
\toprule
& \multirow{2}{*}{Plane}  & \multirow{2}{*}{Car} & \multirow{2}{*}{Bird} & \multirow{2}{*}{ Cat} & \multirow{2}{*}{Deer}  & \multirow{2}{*}{Dog}   & \multirow{2}{*}{Frog} & \multirow{2}{*}{Horse}  & \multirow{2}{*}{Ship}  & \multirow{2}{*}{Truck}   & \multirow{2}{*}{Mean} \\
\\
\midrule
MDiff (ConvNext-s) & 94.5	&	95.8	&	94.2	&	92.1	&	95.5	&	\textbf{98.0}	&	97.5	&	96.5	&	98.2	&	98.1	&		96.0 \\
Ours (ConvNext-s) & \textbf{97.2}	&	\textbf{98.3}	&	\textbf{95.5}	&	\textbf{94.4}	&	\textbf{97.5}	&	96.7	&	\textbf{98.8}	&	\textbf{97.8}	&	\textbf{98.6}	&	\textbf{99.6}	&		\textbf{97.4} \\
\midrule
MDiff (ViT-B) & 94.4	&	95.1	&	90.9	&	89.5	&	93.8	&	94.2	&	97.4	&	95.8	&	96.4	&	96.7	&		94.4\\
Ours (ViT-B) & \textbf{98.0}	&	\textbf{98.7}	&	\textbf{95.6}	&	\textbf{92.7}	&	\textbf{97.1}	&	\textbf{96.3}	&	\textbf{99.0}	&	\textbf{98.1}	&	\textbf{98.8}	&\textbf{	98.8}	&		\textbf{97.3}\\
\bottomrule
\end{tabular}
\caption{\textbf{Comparative evaluation on \oc.} We report the mean of the AUF ($\downarrow$) over five trials. \textbf{Bold} and \underline{underlined} indicate best and second best, respectively. Our method outperforms MDiff regardless of the architecture.}
\label{tab:oneclass}
% }
\end{table*}

\subsection{Pseudo-label accuracy}

We show below that our method is robust against mistakes in the pseudo-labels. We report the AUF on \texttt{Airplane:Rest} under different mistake ratios. Our method stays successful even when pseudo-labels contain errors, with no noticeable loss in performance when pseudo-labels are mislabeled up to $15\%$.

\begin{table}[h]
\caption{AUF ($\downarrow$) on \texttt{Airplane:Rest} with varying pseudo-label accuracy. }
\label{tab:oneclass}
% \resizebox{\linewidth}{!}{
\centering
\setlength{\tabcolsep}{3pt}
\begin{tabular}{c|ccccccc}
\toprule
Fraction correct & 1 & 0.95 & 0.85 & 0.8 & 0.75 & 0.5 & 0 \\
\midrule
AUF & 37 & 39 & 38 & 46 & 49 & 67 & 93\\
\bottomrule
\end{tabular}
% }
\end{table}

\subsection{Full ablation results}

In Tab.~\ref{tab:uood_full} and Tab.~\ref{tab:fewshot_full}, we show the per-experiment results for the tables in the ablation study.

\begin{table*}[t]
\begin{center}
% \resizebox{\textwidth}{!}{
 \begin{tabular}{lccccccccccc}
\toprule
 & \multirow{2}{*}{Plane}  & \multirow{2}{*}{Car} & \multirow{2}{*}{Bird} & \multirow{2}{*}{ Cat} & \multirow{2}{*}{ Deer}  & \multirow{2}{*}{Dog}   & \multirow{2}{*}{Frog} & \multirow{2}{*}{ Horse}  & \multirow{2}{*}{Ship}  & \multirow{2}{*}{Truck} & \multirow{2}{*}{ Average} \\
 \\
\midrule
kNN & 80.0 &  75.5 &  86.3 &  79.6 &  82.7 &  82.4 &  87.7 &  76.5 &  82.4 &  84.3 & 81.7 \\
MahaAD & 86.2 &  78.0 &  89.3 &  88.7 &  85.6 &  80.8 &  92.1 &  79.5 &  90.0 &  90.0 & 86.0 \\
\rowcolor{mygray} MkNN (ours) & \textbf{88.3} &  \textbf{80.3} &  \textbf{89.9} &  \textbf{89.6} &  \textbf{87.3} &  \textbf{84.2} &  \textbf{92.7} &  \textbf{81.9} &  \textbf{90.9} &  \textbf{90.3} & \textbf{87.6} \\
\bottomrule
\end{tabular}
\caption{\textbf{Comparing U-OOD performance on CIFAR10.} We report the AUC over one run as the methods are deterministic. \textbf{Bold} indicates the best method. MkNN is the best scoring function in all ten U-OOD experiments. }
\label{tab:uood_full}
% }
\end{center}
\end{table*}

\begin{table*}[!t]
\begin{center}
% \resizebox{\textwidth}{!}{
 \begin{tabular}{lccccccccccc}
\toprule
 & \multirow{2}{*}{Plane}  & \multirow{2}{*}{Car} & \multirow{2}{*}{Bird} & \multirow{2}{*}{ Cat} & \multirow{2}{*}{ Deer}  & \multirow{2}{*}{Dog}   & \multirow{2}{*}{Frog} & \multirow{2}{*}{ Horse}  & \multirow{2}{*}{Ship}  & \multirow{2}{*}{Truck} & \multirow{2}{*}{ Average} \\
 \\
\midrule
 & \multicolumn{11}{c}{\textit{5-shot}} \\
kNN & 85.8 &  79.8 &  77.5 &  70.4 &  74.6 &  72.0 &  80.5 &  64.6 &  80.4 &  70.7 & 75.6\\
MDiff & 90.2 &  92.1 &  80.0 &  75.5 &  83.0 &  82.6 &  89.7 &  76.1 &  88.9 &  89.1 & 84.7 \\
\rowcolor{mygray} $s^-_{Maha}$ (ours) & 91.7 &  94.4 &  84.7 &  83.3 &  92.2 &  90.5 &  92.4 &  92.4 &  \textbf{94.1} & \textbf{96.4} & 91.2 \\
\rowcolor{mygray} $s^-_{MkNN}$ (ours) & \textbf{93.1} &  \textbf{95.2} &  \textbf{87.0} &  \textbf{84.3} &  \textbf{92.4} &  \textbf{90.7} &  \textbf{92.6} & \textbf{92.6} & 93.5 & 96.3 & \textbf{91.8}\\
\midrule
 & \multicolumn{11}{c}{\textit{10-shot}} \\
kNN & 87.6 &  82.0 &  79.5 &  74.5 &  79.0 &  77.0 &  85.7 &  70.4 &  83.2 &  78.9 & 79.8\\
MDiff & 92.8 &  94.5 &  84.1 &  80.7 &  90.6 &  86.6 &  93.9 &  88.4 &  93.3 &  93.9 & 89.9\\
\rowcolor{mygray} $s^-_{Maha}$ (ours)& 92.5 &  94.8 &  85.7 &  84.2 &  92.8 &  90.9 &  93.5 &  92.5 &  \textbf{95.2} &  96.7 & 91.9 \\
\rowcolor{mygray} $s^-_{MkNN}$ (ours) & \textbf{93.9} &  \textbf{95.7} &  \textbf{87.4} &  \textbf{85.0} &  \textbf{93.7} &  \textbf{91.6} &  \textbf{94.1} &  \textbf{93.2} & \textbf{95.2} & \textbf{96.9} & \textbf{92.7} \\
\bottomrule
\end{tabular}
\caption{\textbf{Comparing few-shot OOD performance on CIFAR10.} We report the mean AUC over five runs. \textbf{Bold} indicates the best method. Our few-shot detector $s^-_{MkNN}$ is best overall. }
\label{tab:fewshot_full}
% }
\end{center}
\end{table*}
